# Supplementary material for: How confused can an entanglement witness be to be still persuasive
Source: arXiv:2011.11340 source file (2020-11-23)
Supplement: Supplementary file 1 [file machine_collectibility_suplement_201112.pdf]

# How confused can an entanglement witness be to be still persuasive: Supplemental materials


Jan Roik,[1,*] Karol Bartkiewicz,[2,1,†] Antonín Černoch,[1,‡] and Karel Lemr[1,§]

[1] *RCPTM, Joint Laboratory of Optics of Palacký University and Institute of Physics of Czech Academy of Sciences, 17. listopadu 12, 771 46 Olomouc, Czech Republic*

[2] *Faculty of Physics, Adam Mickiewicz University, PL-61-614 Poznań, Poland*



(Dated: November 12, 2020)


*State sampling and numerical processing* This paper focuses on general 2-qubit states. In order to correctly prepare test and training data sets, we generate diagonal elements of the $4\times4$ matrix $M$ according to [1]:

$$M = \begin{pmatrix} M_{11} & 0 & 0 & 0 \\ 0 & M_{22} & 0 & 0 \\ 0 & 0 & M_{33} & 0 \\ 0 & 0 & 0 & M_{44} \end{pmatrix} \tag{1}$$

where $M_{11} = r_1$; $M_{22} = r_2(1 - M_{11})$; $M_{33} = r_3(1 - M_{11} - M_{22})$; $M_{44} = r_4(1 - M_{11} - M_{22} - M_{33})$; $r_n$ for $n = 1,2,3,4$ gives uniformly distributed random numbers from range $[0,1]$. The matrix is then normalized. In the next step, proper random unitary transformation was used in order to create a density matrix of general random 2-qubit state [2]

$$\begin{aligned} U = &\begin{pmatrix} 1 & 0 & 0 & 0 \\ 0 & 1 & 0 & 0 \\ 0 & 0 & \multicolumn{2}{c}{\multirow{2}{*}{$U_1$}} \\ 0 & 0 & & \end{pmatrix} \begin{pmatrix} 1 & 0 & 0 & 0 \\ 0 & \multicolumn{2}{c}{\multirow{2}{*}{$U_2$}} & 0 \\ 0 & & & 0 \\ 0 & 0 & 0 & 1 \end{pmatrix} \begin{pmatrix} \multicolumn{2}{c}{\multirow{2}{*}{$U_3$}} & 0 & 0 \\ & & 0 & 0 \\ 0 & 0 & 1 & 0 \\ 0 & 0 & 0 & 1 \end{pmatrix} \\ &\begin{pmatrix} 1 & 0 & 0 & 0 \\ 0 & 1 & 0 & 0 \\ 0 & 0 & \multicolumn{2}{c}{\multirow{2}{*}{$U_4$}} \\ 0 & 0 & & \end{pmatrix} \begin{pmatrix} 1 & 0 & 0 & 0 \\ 0 & \multicolumn{2}{c}{\multirow{2}{*}{$U_5$}} & 0 \\ 0 & & & 0 \\ 0 & 0 & 0 & 1 \end{pmatrix} \begin{pmatrix} 1 & 0 & 0 & 0 \\ 0 & 1 & 0 & 0 \\ 0 & 0 & \multicolumn{2}{c}{\multirow{2}{*}{$U_6$}} \\ 0 & 0 & & \end{pmatrix}, \end{aligned} \tag{2}$$

where

$$U_j = e^{i\alpha_j} \begin{pmatrix} e^{i\psi_j}\cos\phi_j & e^{i\chi_j}\sin\phi_j \\ -e^{-i\chi_j}\sin\phi_j & e^{-i\psi_j}\cos\phi_j \end{pmatrix}, \qquad j = 1,\ldots,6 \tag{3}$$

with $0 \le \phi \le \frac{\pi}{2}, 0 \le \alpha,\psi,\chi < 2\pi$. The homogenous distribution of states was ensured by $\phi_j = \arcsin\sqrt{\xi_j}, \xi_j \in [0,1]$. Parameters $\phi_j,\psi_j,\chi_j,\alpha_j$ and $\xi_j$ are picked from their respective intervals with uniform probability. The final density matrix was obtained as $M_o = UMU^\dagger$. Training and test data were labeled via PPT criterion [3]. To mathematically describe the collective measurement a 4-qubit density matrix $M_f$ was defined as $M_f = M_o \otimes M_t$. To implement Bell-state projection on the neighing $(2,3)$ qubits, $M_t$ is obtained from $M_o$ by switching subsystems

$$M_t = SWAP\ M_0\ SWAP, \tag{4}$$

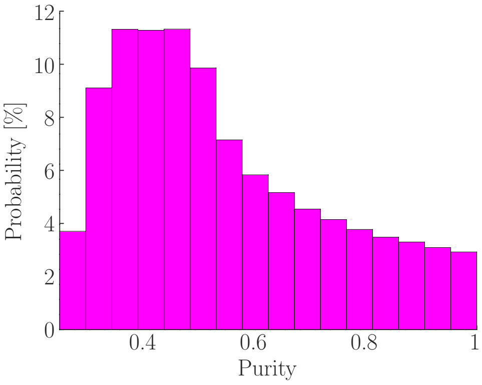


FIG. 1. Purity distribution of the training and test states.

where

$$SWAP = \begin{pmatrix} 1 & 0 & 0 & 0 \\ 0 & 0 & 1 & 0 \\ 0 & 1 & 0 & 0 \\ 0 & 0 & 0 & 1 \end{pmatrix}. \tag{5}$$

*Colectibility.* In order to calculate collectibility we used the formula by Rudnicky *et al.* [4] represented in computational bases, i.e., $H \to |0\rangle$; $V \to |1\rangle$; $D \to |+\rangle = (|0\rangle + |1\rangle)/\sqrt{2}$; $A \to |-\rangle = (|0\rangle - |1\rangle)/\sqrt{2}$; $R \to (|0\rangle - i|1\rangle)/\sqrt{2}$ and, $L \to = (|0\rangle + i|1\rangle)/\sqrt{2}$

$$\begin{aligned} W(\hat{\rho}) = &\frac{1}{2}[\eta + p_0^2(1 - r_{00}) + (1 - p_0)^2(1 - r_{11}) \\ &+ 2p_0(1 - p_0)(1 - r_{01}) - 1], \end{aligned} \tag{6}$$

where

$$\eta = 8p_0(1 - p_0)\sqrt{r_{00}r_{11}} + 2p'. \tag{7}$$

In the equations above single-photon projection probability $p_0 = M_{o_{00}} + M_{o_{11}}$ and $p' = \max\{p_{++}, p_{--}\}$. $P_{xy}$ represents probabilities of single Bell state projection of non-locally measured qubit conditioned on local projection onto $|x\rangle$ and $|y\rangle$ states.[4]

*Other two-copy witnesses.* A class of two-copy entanglement witnesses can be calculated using elements of the symmetric matrix [5]

$$R_{i,j} = R_{j,i} = \left\langle \sigma_i^{(a_1)} \otimes \sigma_j^{(a_2)} \otimes |\Psi^-_{b_1,b_2}\rangle\langle\Psi^-_{b_1,b_2}| \right\rangle, \tag{8}$$

where the expectation values are calculated on two copies of $\rho$, i.e., $\rho_{a_1,b_1} \otimes \rho_{a_2,b_2}$. To estimate the number of projections let use the resolution of two-qubit identity operator valid for an arbitrary $i, j = 1,2,3$, which reads

$$\mathbb{1}^{\otimes 2} = \sum_{r,s=0,1} |r_i s_j\rangle\langle r_i s_j|, \tag{9}$$

where $|0_i\rangle$ and $|1_i\rangle$ are eigenstates of $\sigma_i$ operator associated with $\pm 1$ eigenvalues, respectively. A product of two Pauli operators reads

$$\sigma_i^{(a_1)} \otimes \sigma_j^{(a_2)} = |0_i 0_j\rangle\langle 0_i 0_j| + |1_i 1_j\rangle\langle 1_i 1_j| - (|0_i 1_j\rangle\langle 0_i 1_j| + |1_i 0_j\rangle\langle 1_i 0_j|). \tag{10}$$

By adding the corresponding sides of Eq. (9) to Eq. (10) and subtracting $\mathbb{1}^{\otimes 2}$ we obtain

$$\sigma_i^{(a_1)} \otimes \sigma_j^{(a_2)} = 2(|0_i 0_j\rangle\langle 0_i 0_j| + |1_i 1_j\rangle\langle 1_i 1_j|) - \mathbb{1}^{\otimes 2}. \tag{11}$$

This means that measuring all 6 different elements of $R$ (i.e., $i \le j$ for $i, j = 1,2,3$) requires 12 projections in total. These projections read

$$\begin{gathered} |D\rangle|D\rangle, |A\rangle|A\rangle, |D\rangle|L\rangle, |A\rangle|R\rangle, \\ |D\rangle|H\rangle, |A\rangle|V\rangle, |L\rangle|L\rangle, |R\rangle|R\rangle, \\ |L\rangle|H\rangle, |R\rangle|V\rangle, |H\rangle|H\rangle, |V\rangle|V\rangle. \end{gathered} \tag{12}$$

By using these 12 projections we determine matrix $Q$ used to calculate entanglement witnesses. Fully entangled fraction $f$ can be used to construct an entanglement witness [5]

$$F = 2f - 1 = \tfrac{1}{2}[\mathrm{Tr}(\sqrt{Q}) - 1]. \tag{13}$$

This and the following witnesses are positive, if entanglement is detected and negative, otherwise. The maximum value is 1.

Furthermore, by using an optimal CHSH inequality we can construct an entanglement witness [5] as

$$M = \mathrm{Tr}(Q) - \min[\mathrm{eig}(Q)]. \tag{14}$$

It is also possible to use $Q$ to express an entropic entanglement witness [5]

$$E = \tfrac{1}{2}[\mathrm{Tr}(Q) - 1]. \tag{15}$$


* jan.roik@upol.cz
† bartkiewicz@jointlab.upol.cz
‡ antonin.cernoch@upol.cz
§ k.lemr@upol.cz



[1] J. Maziero, "Random sampling of quantum states: a survey of methods," Brazilian Journal of Physics **45**, 575–583 (2015).


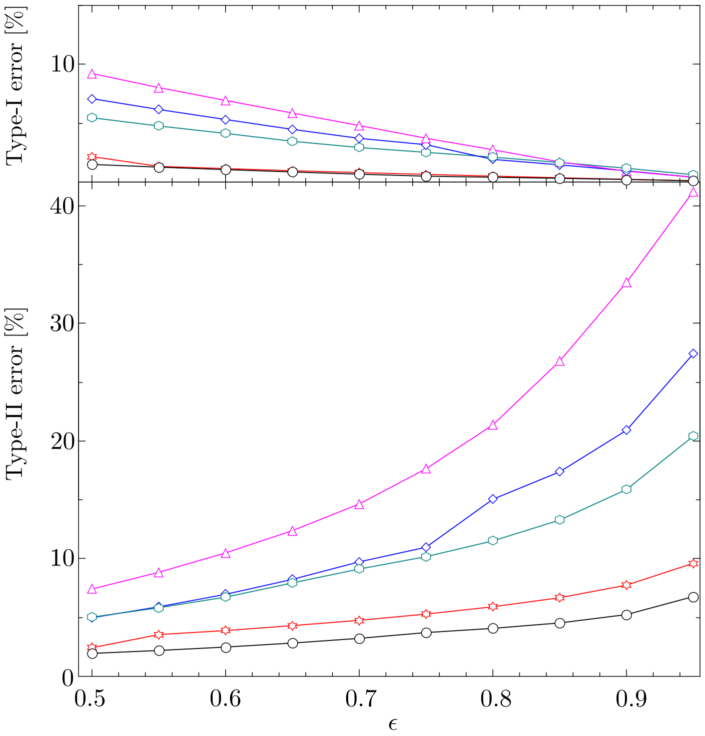


FIG. 2. Dependence of Type I and Type II errors on $\epsilon$ threshold for varying numbers of projections: Three projection $N = 3$ (△), five projections $N = 5$ (◇), six projections $N = 6$ (⬠), twelve projections $N = 12$ (☆), fifteen projections $N = 15$ (○).

| N | $\vert i\rangle\vert j\rangle$ |
|---|---|
| 3 | $\vert H\rangle\vert H\rangle, \vert V\rangle\vert V\rangle, \vert H\rangle\vert V\rangle$ |
| 5 | $\vert H\rangle\vert H\rangle, \vert V\rangle\vert V\rangle, \vert H\rangle\vert V\rangle, \vert D\rangle\vert D\rangle, \vert A\rangle\vert A\rangle$ |
| 6 | $\vert H\rangle\vert H\rangle, \vert V\rangle\vert V\rangle, \vert H\rangle\vert V\rangle, \vert D\rangle\vert D\rangle, \vert R\rangle\vert R\rangle, \vert L\rangle\vert L\rangle$ |
| 12 | $\vert D\rangle\vert D\rangle, \vert A\rangle\vert A\rangle, \vert D\rangle\vert L\rangle, \vert A\rangle\vert R\rangle, \vert D\rangle\vert H\rangle, \vert A\rangle\vert V\rangle,$ $\vert L\rangle\vert L\rangle, \vert R\rangle\vert R\rangle, \vert L\rangle\vert H\rangle, \vert R\rangle\vert V\rangle, \vert H\rangle\vert H\rangle, \vert V\rangle\vert V\rangle,$ |
| 15 | $\vert D\rangle\vert D\rangle, \vert A\rangle\vert A\rangle, \vert D\rangle\vert L\rangle, \vert A\rangle\vert R\rangle, \vert D\rangle\vert H\rangle, \vert A\rangle\vert V\rangle, \vert L\rangle\vert L\rangle,$ $\vert R\rangle\vert R\rangle, \vert L\rangle\vert H\rangle, \vert R\rangle\vert V\rangle, \vert H\rangle\vert H\rangle, \vert V\rangle\vert V\rangle, \vert D\rangle\vert R\rangle, \vert D\rangle\vert V\rangle, \vert L\rangle\vert V\rangle$ |

TABLE I. List of specific projections settings used for the learning of the artificial neural network.

| N | 3 | | 5 | | 6 | | 12 | | 15 | |
|---|---|---|---|---|---|---|---|---|---|---|
| $\epsilon$ | T-I | T-II | T-I | T-II | T-I | T-II | T-I | T-II | T-I | T-II |
| 0.5 | 9.23 | 7.42 | 7.09 | 4.98 | 5.47 | 5.03 | 2.17 | 2.43 | 1.50 | 1.94 |
| 0.55 | 8.03 | 8.84 | 6.17 | 5.91 | 4.77 | 5.83 | 1.34 | 3.55 | 1.27 | 2.19 |
| 0.6 | 6.94 | 10.49 | 5.32 | 6.97 | 4.14 | 6.73 | 1.15 | 3.89 | 1.06 | 2.48 |
| 0.65 | 5.87 | 12.38 | 4.48 | 8.24 | 3.47 | 7.94 | 0.97 | 4.31 | 0.86 | 2.82 |
| 0.7 | 4.81 | 14.65 | 3.72 | 9.73 | 2.94 | 9.12 | 0.81 | 4.76 | 0.67 | 3.22 |
| 0.75 | 3.73 | 17.64 | 3.18 | 10.97 | 2.53 | 10.17 | 0.66 | 5.29 | 0.50 | 3.71 |
| 0.8 | 2.75 | 21.37 | 1.93 | 15.05 | 2.12 | 11.51 | 0.51 | 5.91 | 0.41 | 4.07 |
| 0.85 | 1.72 | 26.79 | 1.47 | 17.38 | 1.67 | 13.28 | 0.37 | 6.68 | 0.32 | 4.53 |
| 0.9 | 0.93 | 33.47 | 0.96 | 20.91 | 1.18 | 15.88 | 0.24 | 7.75 | 0.22 | 5.24 |
| 0.95 | 0.41 | 41.21 | 0.42 | 27.42 | 0.63 | 20.41 | 0.11 | 9.61 | 0.11 | 6.77 |

TABLE II. Evolution of Type-I and Type-II error for different thresholds $\epsilon$. T-I and T-II represent Type-I and Type-II errors respectively and are listed in percentages.

[2] C.-K. LI, R. ROBERTS, and X. YIN, "Decomposition of unitary matrices and quantum gates," International Journal of Quantum Information **11**, 1350015 (2013), https://doi.org/10.1142/S0219749913500159.

[3] R. Simon, "Peres-Horodecki separability criterion for continuous variable systems," Phys. Rev. Lett. **84**, 2726–2729 (2000).

[4] Ł. Rudnicki, Z. Puchała, P. Horodecki, and K. Życzkowski, "Collectibility for mixed quantum states," Phys. Rev. A **86**, 062329 (2012).

[5] Karol Bartkiewicz, Karel Lemr, Antonín Černoch, and Adam Miranowicz, "Bell nonlocality and fully entangled fraction measured in an entanglement-swapping device without quantum state tomography," Phys. Rev. A **95**, 030102 (2017).
